# Supplementary material for: Spaced Repetition and Mnemonics Enable Recall of Multiple Strong Passwords
Source: arXiv:1410.1490 source file (2020-01-24)
Supplement: Supplementary file 1 [file Appendix.tex]

\subsection{List of People, Actions and Objects from the User Study} \label{subsec:ListOfPAO}

Here are a list of the people, actions and objects we used in the study. The lists contain $92$ actions and $96$ objects respectively.

\noindent{\bf People:} Ben Afleck, Beyonce, Joe Biden, Kobe Bryant, George W Bush, Bill Clinton, Hillary Clinton, Albert Einstein, Jimmy Fallon, Pope Francis, Frodo, Gandalf, Bill Gates, Adolf Hitler,  Lebron James, Steve Jobs, Angelina Jolie,  Michael Jordan,  Nelson Mandela,  Barack Obama, Rand Paul, Ron Paul, Michael Phelps, Brad Pitt, Bart Simpson, Homer Simpson, Luke Skywalker, Justin Timberlake, Kim Jong Un, Darth Vader, Oprah Winfrey, Tiger Woods, Jay Z, Mark Zuckerberg

\noindent{\bf Actions:} aiming, aligning,  batting,  bowing, bribing, burying, canning, chipping, choking, climbing,  coating, combing, concealing,  cooking,  copying,  destroying,   dodging, drying, dueling,  egging, elbowing,  fanning,  firing, fishing,  flying,  following,  fuming, giving, gluing, gnawing,   high fiving, howling, hunting,  inhaling, judging, juicing,  jumping, kicking, kissing,  knifing,  lassoing,  leashing,  muddying, miming, marrying, mauling, mashing, mugging, moving, mopping, mowing, nipping,  nosing,  numbing, oiling, paddling, plowing, popping, puking, pulling,  punching, racing, raking, reaching, reeling, riding, rolling, rowing, saving, searing, seizing, sheering, shining,  signing, sipping, smelling, stewing, stretching, sucking, swallowing, swimming, taping, tasting, tattooing, tazing, tugging, voting, waking, waving,  weeping, welding

\noindent{\bf Objects:} ammo, ant, apple, arrow, beehive, bike, boa, boar, bomb, bunny, bus, bush, cab, cake, canoe, cat, chain, chainsaw, cheese, cheetah, chili, chime, coffee, couch, cow, daisy, dime, dish, ditch, dove, duck, fish, foot, goose, gyro, hammer, hen, home, hoof, horse, igloo, iron, jeep, jet, key, kite, leach, leaf, lime, lion, lock, mail, 
menu, microphone, moon, moose, mummy, nail, navy, nose, onion, owl, patty, phone, pill, pin, piranha, puppy, ram, rat, razor-blade, rib, roach, safe, sauce, saw, seal, shark, shoe, shoe, snake, snow, soap, sock, suit, sumo, teacup, tepee, tiger, tire, toad, toe, vase, waffle, wagon, wiener
